# Supplementary material for: Just Label What You Need: Fine-Grained Active Selection for Perception and Prediction through Partially Labeled Scenes
Source: arXiv:2104.03956 source file (2021-04-08)
Supplement: Supplementary file 1 [file supplementary_examples.tex]

\begin{figure*}[ht!]
     \includegraphics[width=.37\textwidth]{figures/supplementary/qualitative_examples/cfa8b6df-8cb6-4bb6-fa30-6185979beb9a_40.png} \hspace{-0.8cm}
     \includegraphics[width=.37\textwidth]{figures/supplementary/qualitative_examples/cc437640-a3fd-4c71-ee17-48aa4c0c4a8b_40.png} \hspace{-0.8cm}
     \includegraphics[width=.37\textwidth]{figures/supplementary/qualitative_examples/c5b1af99-1631-413e-c64d-77935cbf1d80_140.png}
     \includegraphics[width=.37\textwidth]{figures/supplementary/qualitative_examples/dc181e4a-08ae-41d4-c6fa-535f766c6336_100.png} \hspace{-0.8cm}
     \includegraphics[width=.37\textwidth]{figures/supplementary/qualitative_examples/d8ed7d11-a493-40bb-e417-4d123ea3d352_80.png} \hspace{-0.8cm}
     \includegraphics[width=.37\textwidth]{figures/supplementary/qualitative_examples/d00ec90a-caa0-44f6-ee3f-d5f2239f8e5c_20.png}
     \includegraphics[width=.37\textwidth]{figures/supplementary/qualitative_examples/000dfbf5-a60e-4a49-c1c6-eedd218d559f_180.png} \hspace{-0.8cm}
     \includegraphics[width=.37\textwidth]{figures/supplementary/qualitative_examples/ff258e62-2f54-459d-ff87-017b8e634c79_140.png} \hspace{-0.8cm}
     \includegraphics[width=.37\textwidth]{figures/supplementary/qualitative_examples/fa5fb00d-d0ab-4060-c819-dc56a2e69f51_80.png}
     \includegraphics[width=.37\textwidth]{figures/supplementary/qualitative_examples/f475e120-8cc3-4189-e3ec-26495adb8916_60.png} \hspace{-0.8cm}
     \includegraphics[width=.37\textwidth]{figures/supplementary/qualitative_examples/f2a4f946-90db-41ec-eb12-d86b740e41b3_80.png} \hspace{-0.8cm}
     \includegraphics[width=.37\textwidth]{figures/supplementary/qualitative_examples/edaebcf4-5cd1-40c1-de83-f7ee07e6d92a_80.png}
     \includegraphics[width=.37\textwidth]{figures/supplementary/qualitative_examples/e7d10196-92a4-426e-ea99-2c220ea92c0d_120.png} \hspace{-0.8cm}
     \includegraphics[width=.37\textwidth]{figures/supplementary/qualitative_examples/e6a0c17b-cbcd-4e7c-f17f-f0cd833b7a94_80.png} \hspace{-0.8cm}
     \includegraphics[width=.37\textwidth]{figures/supplementary/qualitative_examples/e6a0c17b-cbcd-4e7c-f17f-f0cd833b7a94_100.png}
     \includegraphics[width=.37\textwidth]{figures/supplementary/qualitative_examples/e42f6e9b-3b6c-454a-f1ca-95b8fc7d4941_100.png} \hspace{-0.8cm}
     \includegraphics[width=.37\textwidth]{figures/supplementary/qualitative_examples/e1ebb4a4-8d71-4424-da4c-8ae90e280c84_40.png} \hspace{-0.8cm}
     \includegraphics[width=.37\textwidth]{figures/supplementary/qualitative_examples/e05db1be-0ec4-4fde-edaa-8e1d9185e918_20.png}
 \end{figure*}

 \begin{figure*}[ht!]
     \includegraphics[width=.37\textwidth]{figures/supplementary/qualitative_examples/7c995281-75a7-44c7-dc83-83c2d3abde8e_20.png} \hspace{-0.8cm}
     \includegraphics[width=.37\textwidth]{figures/supplementary/qualitative_examples/7a62ae68-089f-427b-e19d-54c6b47bfb3a_80.png} \hspace{-0.8cm}
     \includegraphics[width=.37\textwidth]{figures/supplementary/qualitative_examples/7848d3e5-64b2-48bc-e5eb-d9c5d1e89464_100.png}
     \includegraphics[width=.37\textwidth]{figures/supplementary/qualitative_examples/8b594800-1ee9-4ff5-fecb-723799c2508d_40.png} \hspace{-0.8cm}
     \includegraphics[width=.37\textwidth]{figures/supplementary/qualitative_examples/8422d43b-79be-4a1d-c1be-1921d57f934f_120.png} \hspace{-0.8cm}
     \includegraphics[width=.37\textwidth]{figures/supplementary/qualitative_examples/82c0e71d-ebd6-4b50-fc2b-b139dafefbe3_60.png}
     \includegraphics[width=.37\textwidth]{figures/supplementary/qualitative_examples/8f11312f-22c3-4597-ffd9-65d25adf71ca_80.png} \hspace{-0.8cm}
     \includegraphics[width=.37\textwidth]{figures/supplementary/qualitative_examples/8ee68d59-d1b5-442e-e5ea-9b63927a9109_20.png} \hspace{-0.8cm}
     \includegraphics[width=.37\textwidth]{figures/supplementary/qualitative_examples/8c7c9354-5877-470b-e8d2-48883e40b442_80.png}
     \includegraphics[width=.37\textwidth]{figures/supplementary/qualitative_examples/97aa7735-9037-4f3a-c7c9-2130188764e6_40.png} \hspace{-0.8cm}
     \includegraphics[width=.37\textwidth]{figures/supplementary/qualitative_examples/97aa7735-9037-4f3a-c7c9-2130188764e6_140.png} \hspace{-0.8cm}
     \includegraphics[width=.37\textwidth]{figures/supplementary/qualitative_examples/9170c8c9-2f49-4ac5-c734-92f0e373102b_120.png}
     \includegraphics[width=.37\textwidth]{figures/supplementary/qualitative_examples/99ac926e-18b4-45d1-dd96-a7429817fddb_160.png} \hspace{-0.8cm}
     \includegraphics[width=.37\textwidth]{figures/supplementary/qualitative_examples/995bbb21-a5d9-432a-c801-26d30ee7afa2_180.png} \hspace{-0.8cm}
     \includegraphics[width=.37\textwidth]{figures/supplementary/qualitative_examples/98d9d8e9-7b86-4beb-eea4-a403a0af23e1_100.png}
     \includegraphics[width=.37\textwidth]{figures/supplementary/qualitative_examples/a0b91cab-c654-465d-f5ed-741a9f58a4db_40.png} \hspace{-0.8cm}
     \includegraphics[width=.37\textwidth]{figures/supplementary/qualitative_examples/9fa10e94-23fa-4a57-c4a8-7ce82f1bfe87_40.png} \hspace{-0.8cm}
     \includegraphics[width=.37\textwidth]{figures/supplementary/qualitative_examples/9d7a55b1-315c-457d-fdd7-b829d6c31fe6_80.png}
     \includegraphics[width=.37\textwidth]{figures/supplementary/qualitative_examples/a522eafc-d526-49ba-f725-fe75ee91c431_120.png} \hspace{-0.8cm}
     \includegraphics[width=.37\textwidth]{figures/supplementary/qualitative_examples/a38ededc-49e6-4b5e-fa4d-af16c38ca4e3_80.png} \hspace{-0.8cm}
     \includegraphics[width=.37\textwidth]{figures/supplementary/qualitative_examples/a3729b7c-2317-4179-c46e-e1e17999199f_20.png}
 \end{figure*}

 \begin{figure*}[ht!]

         \includegraphics[width=.37\textwidth]{figures/supplementary/qualitative_examples/402b345b-d87a-4046-dd7c-dcf79f65e81c_120.png} \hspace{-0.8cm}
         \includegraphics[width=.37\textwidth]{figures/supplementary/qualitative_examples/3cd7df4c-9a09-42a5-ee2f-cc442e52869d_20.png} \hspace{-0.8cm}
         \includegraphics[width=.37\textwidth]{figures/supplementary/qualitative_examples/34c72404-ccc7-4bfa-d54d-3f4af1527b7a_40.png}
         \includegraphics[width=.37\textwidth]{figures/supplementary/qualitative_examples/4c3bf01d-48c5-4ee4-f828-1f3165632116_100.png} \hspace{-0.8cm}
         \includegraphics[width=.37\textwidth]{figures/supplementary/qualitative_examples/4838c435-8c0b-4dda-eb74-f9bde9e94105_160.png} \hspace{-0.8cm}
        \includegraphics[width=.37\textwidth]{figures/supplementary/qualitative_examples/bb23ea01-ef08-4afc-fa91-b9d6af3e1463_40.png} \hspace{-0.8cm}
         \includegraphics[width=.37\textwidth]{figures/supplementary/qualitative_examples/4d8646f5-d35b-4b63-cf3c-f760b6eb4b3b_40.png} \hspace{-0.8cm}
         \includegraphics[width=.37\textwidth]{figures/supplementary/qualitative_examples/4d561451-1304-42a3-c340-8d5265bf2460_120.png} \hspace{-0.8cm}
         \includegraphics[width=.37\textwidth]{figures/supplementary/qualitative_examples/4cab7196-58c6-4792-c450-b9411aec1568_120.png}
         \includegraphics[width=.37\textwidth]{figures/supplementary/qualitative_examples/5855c450-3edf-4914-ca57-96826939206f_120.png} \hspace{-0.8cm}
         \includegraphics[width=.37\textwidth]{figures/supplementary/qualitative_examples/54de46fd-f200-40b5-f98e-12103937e0a4_80.png} \hspace{-0.8cm}
         \includegraphics[width=.37\textwidth]{figures/supplementary/qualitative_examples/50197b5a-dd24-4385-dd1d-c681090f0835_100.png}
         \includegraphics[width=.37\textwidth]{figures/supplementary/qualitative_examples/5eae2576-f851-4ed7-c1ec-fac7e04af689_120.png} \hspace{-0.8cm}
         \includegraphics[width=.37\textwidth]{figures/supplementary/qualitative_examples/5ce4002b-5bdd-4c48-ff13-ad9ace7df53e_60.png} \hspace{-0.8cm}
         \includegraphics[width=.37\textwidth]{figures/supplementary/qualitative_examples/5bb40f60-24b6-4561-d366-78f697a4ef54_120.png}
         \includegraphics[width=.37\textwidth]{figures/supplementary/qualitative_examples/68ed2a8d-bb48-4ad3-f0c5-4a73dd41a9c7_120.png} \hspace{-0.8cm}
         \includegraphics[width=.37\textwidth]{figures/supplementary/qualitative_examples/67cb7a09-b1f6-44b9-d429-2aabdcecfc09_120.png} \hspace{-0.8cm}
         \includegraphics[width=.37\textwidth]{figures/supplementary/qualitative_examples/6317133d-6682-40de-d605-96e4aa9a7c5a_180.png}
         \includegraphics[width=.37\textwidth]{figures/supplementary/qualitative_examples/75a9e309-3dda-4a59-f6b4-1cc42393b4ac_120.png} \hspace{-0.8cm}
         \includegraphics[width=.37\textwidth]{figures/supplementary/qualitative_examples/7230278c-b23c-47b1-f4c2-f51f1836e76b_140.png} \hspace{-0.8cm}
         \includegraphics[width=.37\textwidth]{figures/supplementary/qualitative_examples/6bd0b9fb-972d-4044-ff8a-d19319c458fd_20.png}
 \end{figure*}
